# Supplementary material for: Dialogizer: Context-aware Conversational-QA Dataset Generation from Textual Sources
Source: arXiv:2311.07589 source file (2023-11-09)
Supplement: Supplementary file 1 [file Figure_Instruction.tex]

\begin{figure*}[t]
\centering
\includegraphics[width=0.8\textwidth]{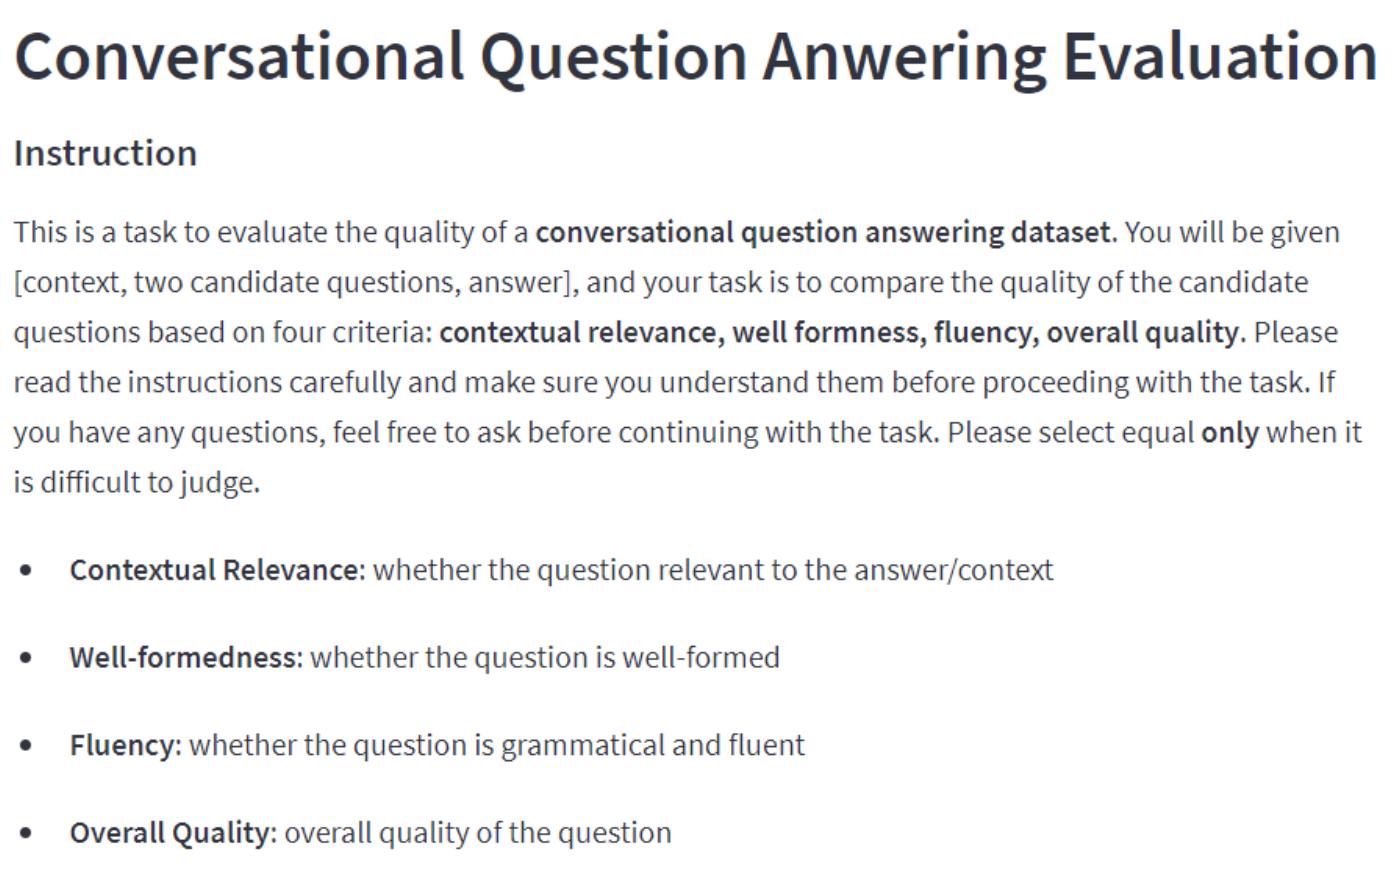} 
\caption{Instruction}
\label{fig_instruction}
\end{figure*}
